# Supplementary material for: Predictive Display with Perspective Projection of Surroundings in Vehicle Teleoperation to Account Time-delays
Source: arXiv:2211.11918 source file (2022-11-22)
Supplement: Supplementary file 1 [file appendixA.tex]

\section*{Appendix A}
\begin{center}
    Errors associated in process flow of PP
\end{center}
\subsubsection{Depth-map to point-cloud conversion}
At control-station, depth-map decoding pertains to error. Depth decoding error is proportional to the depth itself as per figure \ref{fig:x linear}. E.g., error for depth of 1m is 1cm.

\begin{figure}[h]
\centering
\begin{subfigure}[b]{0.243\textwidth}
    \centering
    \includegraphics[width=\textwidth]{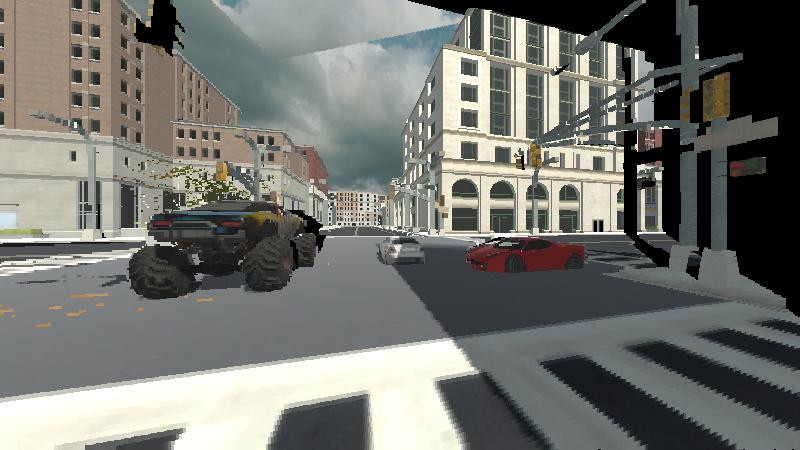}
    \caption{Perspective projection using raw depth-map}
    \label{fig:x depthRaw}
\end{subfigure}%
\hfill
\begin{subfigure}[b]{0.243\textwidth}
    \centering
    \includegraphics[width=\textwidth]{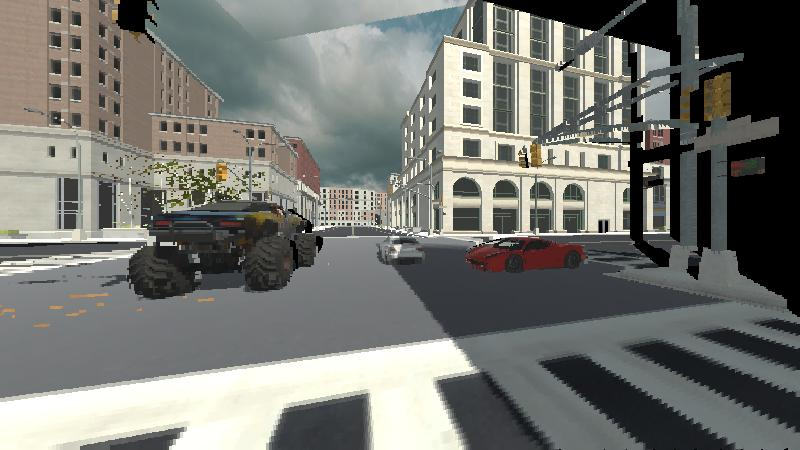}
    \caption{Perspective projection using encoded depth-map}
    \label{fig:x depthEncoded}
\end{subfigure}
\caption{Comparison between perspective projection using raw depth-map vs using encoded depth-map}
\label{fig:x depthCompressionEffect}
\end{figure}

By comparing figures \ref{fig:x depthRaw} and \ref{fig:x depthEncoded}, it has been found that buildings have moved little closer. This is because of (uint8) integer overflow in encoding depths which are more than 20m. But accurate perspective is obtained for closer objects such as the vehicles. During vehicle teleoperation, closer objects are of more interest than farther objects, this trade-off is acceptable to save network bandwidth.

\begin{figure}[h]
    \centering
    \includegraphics[width=0.48\textwidth]{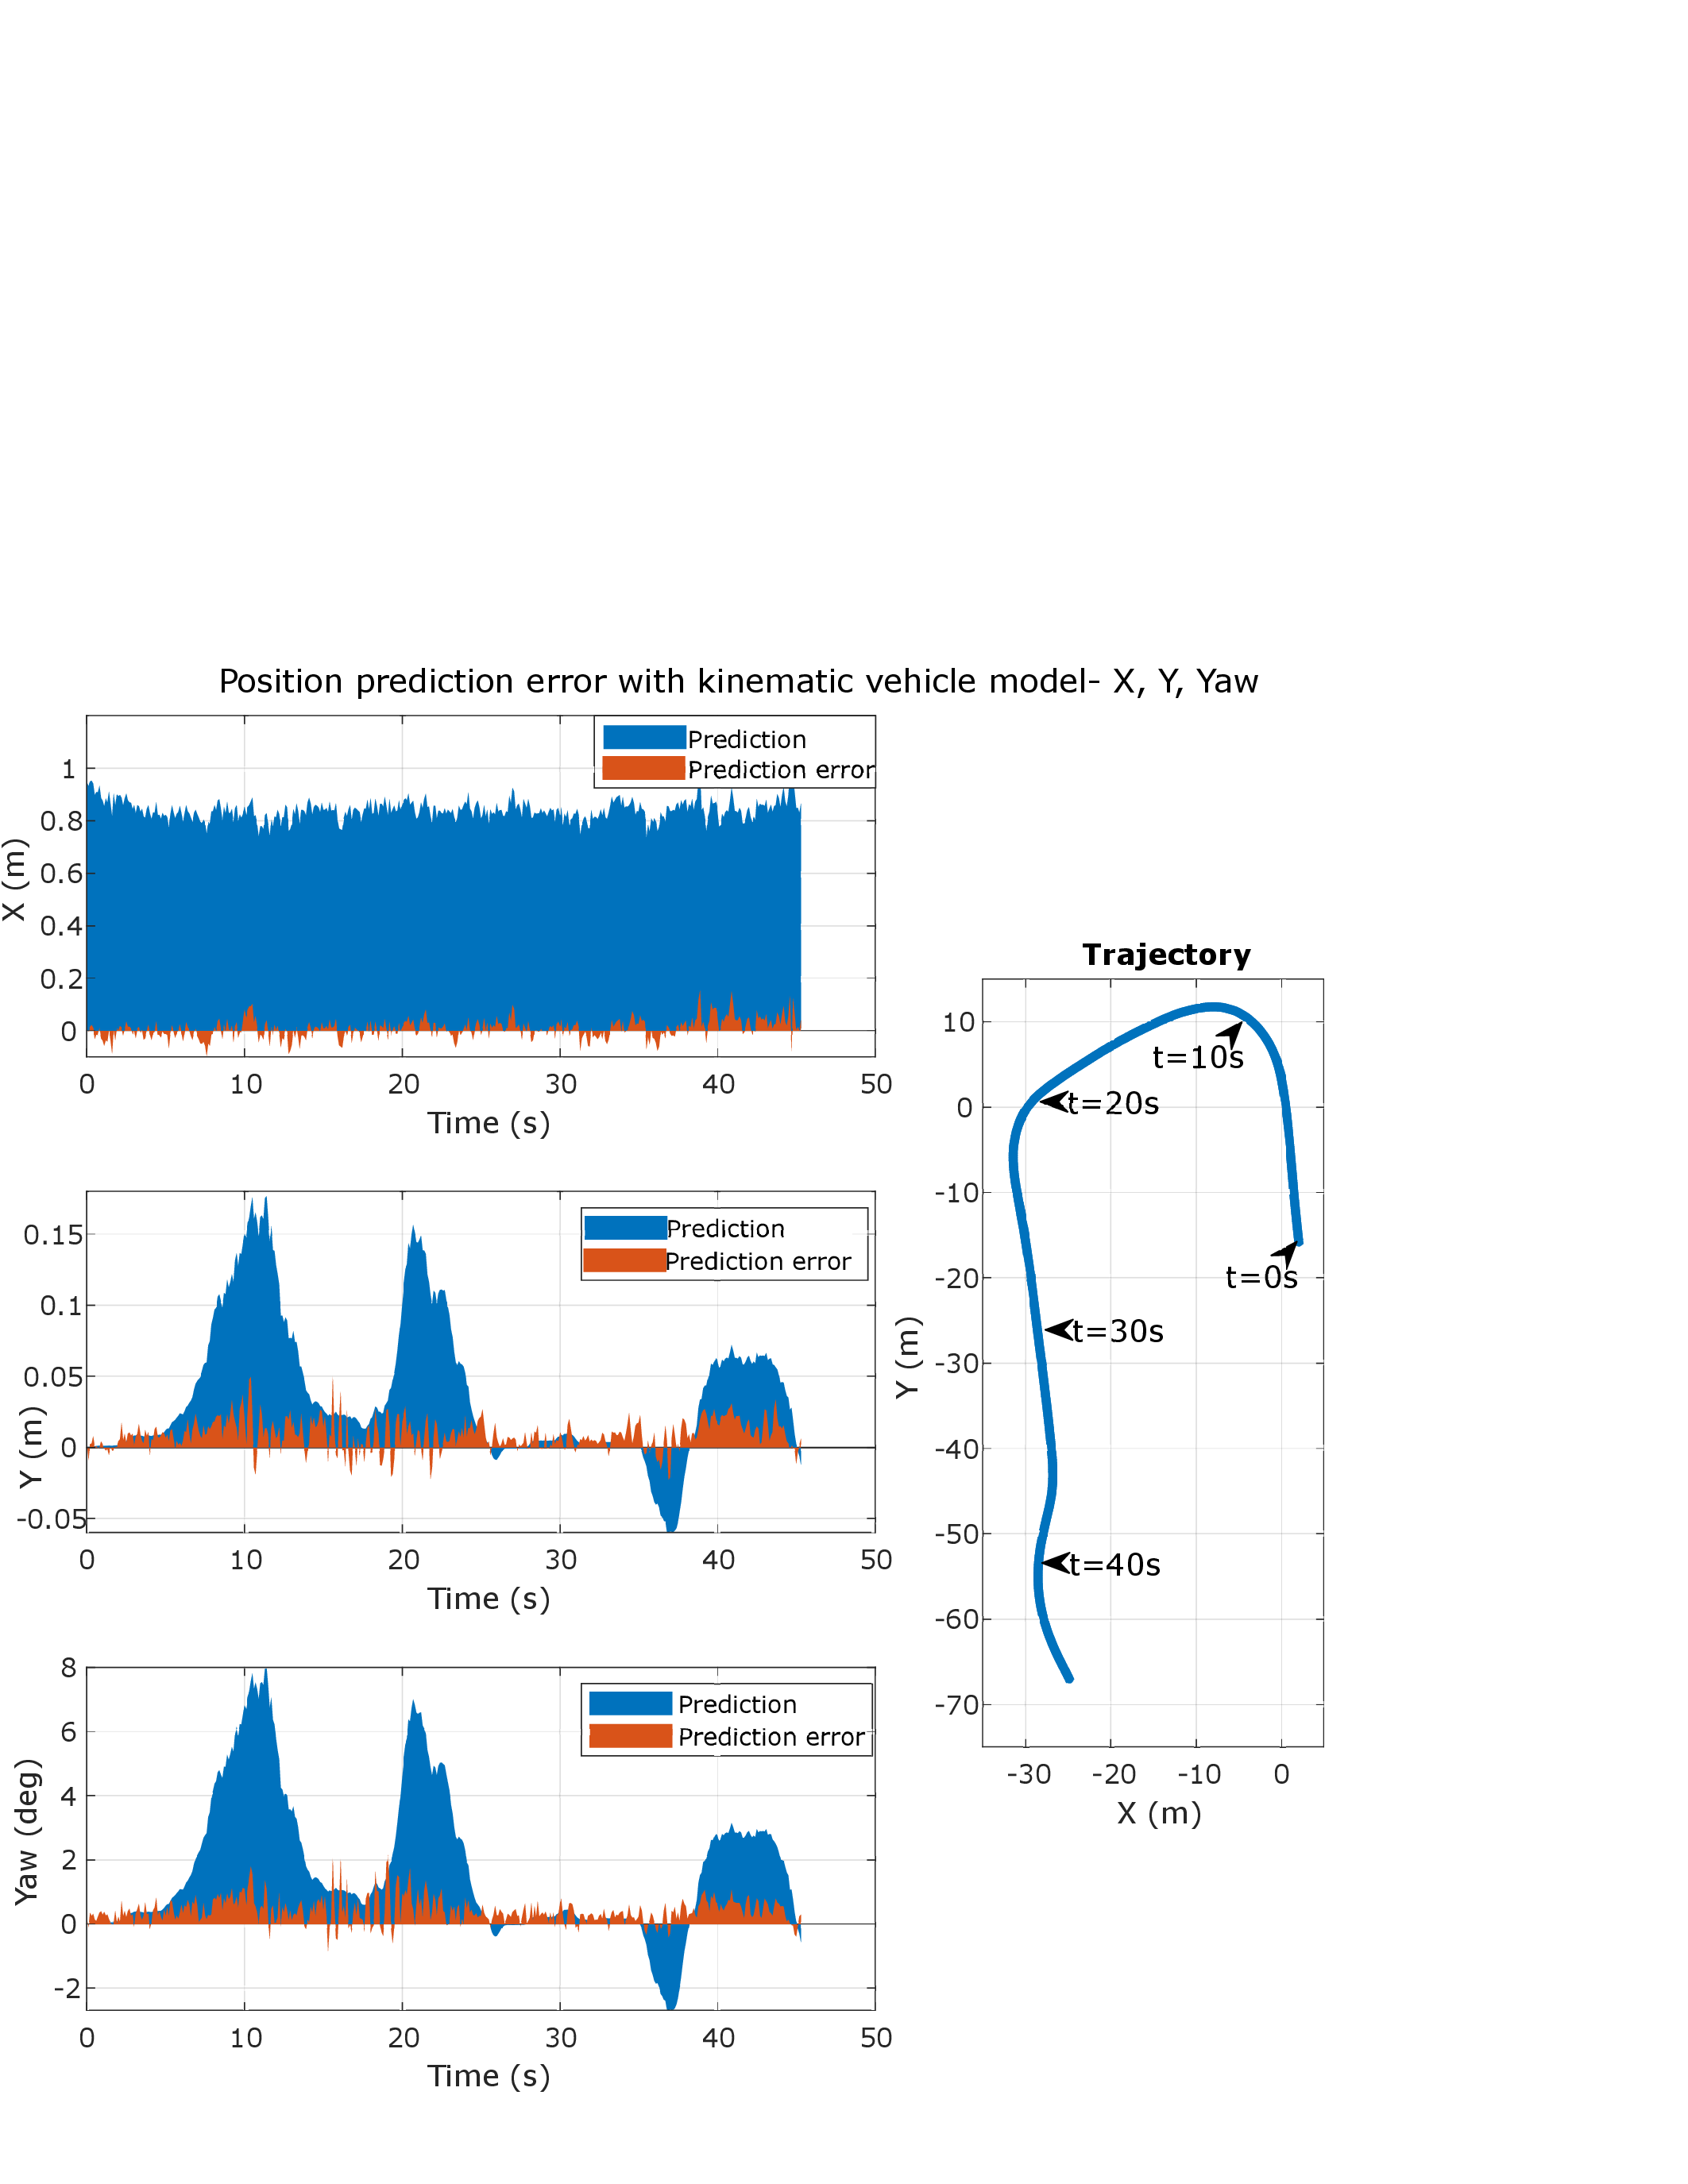}
    \caption{Prediction error of kinematic vehicle model}
    \label{fig:x 0_predictionError}
\end{figure}
\subsubsection{Point-cloud transformation }
Here, factor of error is vehicle model inefficiency in integrating the trajectory for the delay time ($\sim250$ms). The kinematic vehicle model is predicting the vehicle pose with respect to the delayed pose accounting the delay and vehicle speed. Figure \ref{fig:x 0_predictionError}, presents the predicted pose ($X, Y and \:Yaw$) and corresponding errors during \textit{TeleOp with PP-Lap 1} (animation in \textit{Video2} of supplemental files). The error is the difference in predicted pose and actual pose realised by the vehicle after the considered delay. Table \ref{tab:rmseY} presents the RMS error in lateral direction for different time sections. The percentage error is more during lane change manoeuver, which caused due to unaccounted lateral slip by the kinematic vehicle model. The vehicle model is predicting more lateral movement compare to actual lateral movement in presence of under-steering behaviour. Also, the relatively more percent error correspond to the section (38-45s) where the steer changes its sign to be in the second lane. A dynamic single track model can be used to reduce this error.

\begin{table}[h]
\centering
\caption{Lateral error observed in respective manoeuver}
\label{tab:rmseY}
\begin{tabular}{|c|c|}
\hline
\textbf{Time section} & \textbf{RMSE Y} \\ \hline
6-15s                  & 18cm             \\ \hline
19-24s                 & 14cm             \\ \hline
35-38s                 & 12cm             \\ \hline
38-45s                 & 18cm             \\ \hline
\end{tabular}
\end{table}

\subsubsection{Point-cloud to depth-map conversion & Pixel scaling}
These steps are responsible to place objects back on the 2D-image plane of the predicted cam-position. Due to fact that pixels are discrete in nature, error here is $\pm0.5$ pixel.

\subsubsection{RGB mapping}
This step is copying the colour information of the objects; it doesn’t add additional error in the process flow.
